# Supplementary material for: Towards Adversarial Robustness And Backdoor Mitigation in SSL
Source: arXiv:2403.15918 source file (2024-09-16)
Supplement: Supplementary file 1 [file cluster.tex]

\subsection{Visualizing poison distribution in learned representation spaces}

Here, we demonstrate through scatter plots how the poisoned embeddings are distributed with respect to the complete data landscape for CIFAR 10. For the CIFAR 10 test dataset (10,000 images, 1000 images per class), we randomly sample 1000 indices and poison these images. We use a combination of PCA (n\_components = 50) followed by a t-SNE dimensionality reduction to represent the data in two dimensions. We observe that the poison embeddings greatly overlap with the target class in the `RGB` case(s) (Fig. \ref{fig:clusters1}, \ref{fig:clusters2}), making the backdoor attack quite effective. However, in case of Luma, the poison embeddings appear distributed across the data landscape in a disjointed fashion. This indicates failure of backdoor attack, and demonstrates a visual reasoning behind the success of our defense. 

\begin{figure}[tp]
    \centering
    \begin{minipage}[b]{0.24\textwidth}
        \centering
        \includegraphics[width=\textwidth]{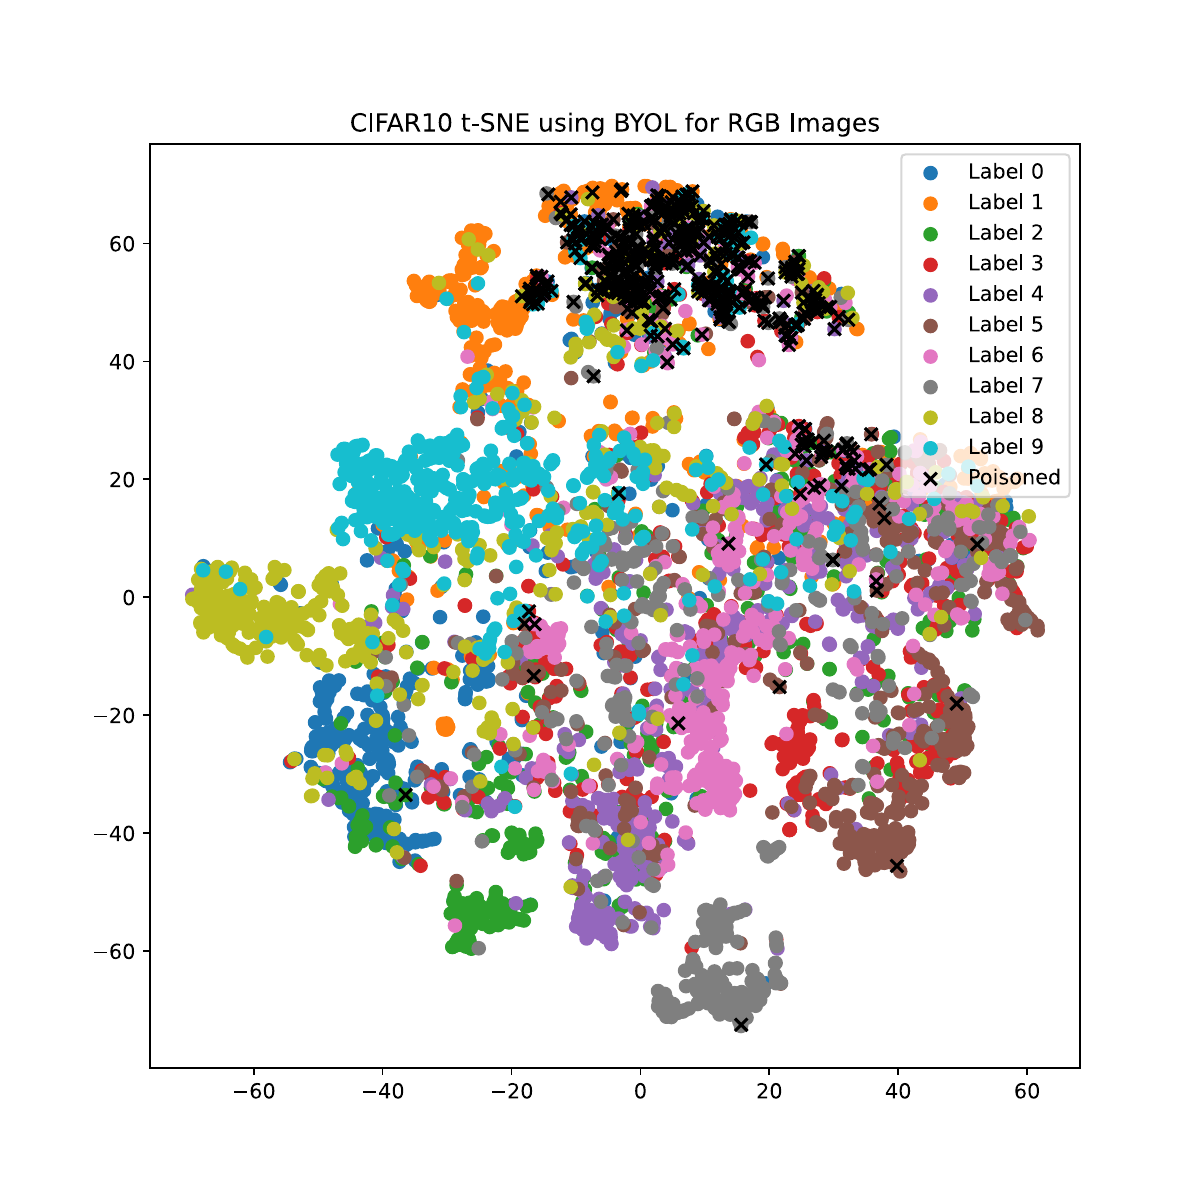}
    \end{minipage}
    \hspace{-1em}
    \begin{minipage}[b]{0.24\textwidth}
        \centering
        \includegraphics[width=\textwidth]{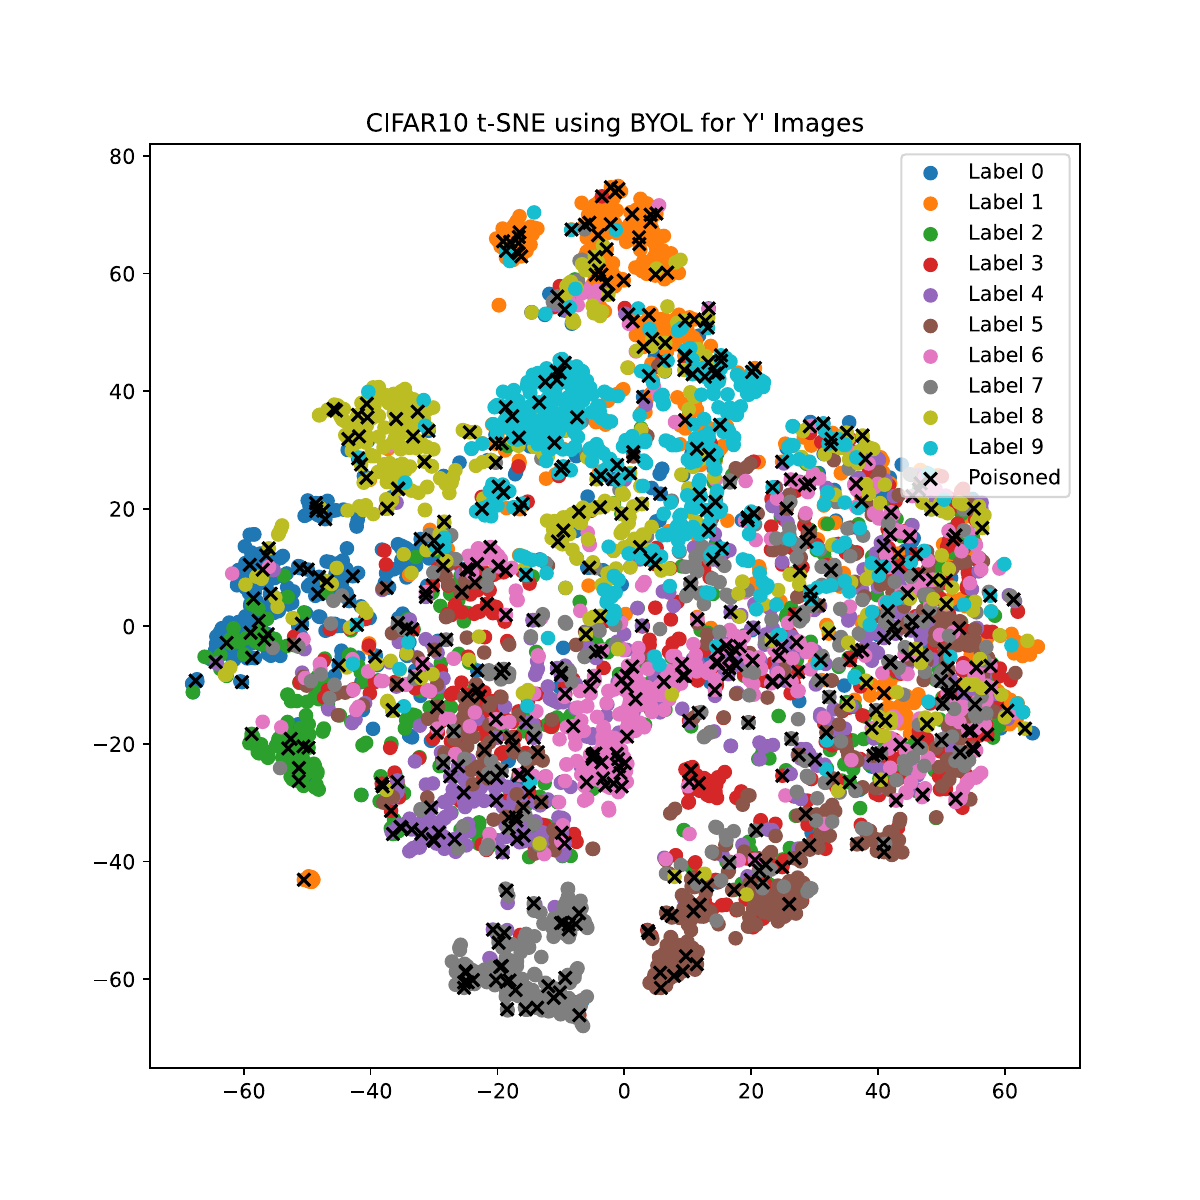}
    \end{minipage}
    \caption{t-SNE Clustering on BYOL using (left) RGB images display the attack, (right) Y’ images display the defense.}
    \label{fig:clusters2}
\end{figure}

%% Aryan
% 1: suggest replace "10000" with "10,000"
% 2: simply write the acronym for t-SNE
% 3: suggest rephrase "for the Y' case(s)" as "In case of Luma"
% 4: suggest rephrasing "results in the backdoor failing" as "indicates failure of backdoor attack"  %Accept
