# Supplementary material for: Towards Adversarial Robustness And Backdoor Mitigation in SSL
Source: arXiv:2403.15918 source file (2024-09-16)
Supplement: Supplementary file 2 [file ctrl.tex]

\subsection{CTRL}
CTRL, introduced in \cite{CTRL}, is a frequency-based poisoning attack targetting SSL. The attack solves two pitfalls faced by attacks introduced in prior work: (a) invariance to augmentations and  (b) reasonable evasiveness (invisible to the human eye). Let $x$ be an image to be poisoned, they separate $Y'UV$ channels of image ($x_{Y'}$, $x_{U}$, $x_{V}$). In order to solve (b), the trigger is only added in $UV$ channels, leaving $Y'$ untouched, thereby rendering it imperceptible to the human eye (Sec. \ref{subsec:luma}). To solve (a), they find Fast Fourier Transform (fft) of $x_U$, $x_V$, and perturb in that space.
\vspace{0.2ex}
\begin{gather}
    \begin{aligned}
    & x^f_U: && \text{FFT}(x_U)
    &&\text{\hspace{1em}}&&
    & x^f_V: && \text{FFT}(x_V)
    % \label{eq:wml-1}
    \end{aligned}
\end{gather}

\vspace{0.2ex}
The trigger $t$ is defined in \cite{CTRL} as
\vspace{0.2ex}
\begin{equation}
t_{i, j} = 
\left
\{\begin{array}{c l}
c & \quad \text{when } i = j \text{ and } i \in \{\frac{s}{2}, s\}\\
0 & \quad \text{otherwise}
\end{array} .
\right.
\end{equation}

\vspace{0.2ex}
where $c$ called magnitude, represents the strength of the poison, and $s$ represents image size (32 for CIFAR 10 and 100). The poisoned sample $y$ is obtained as

\vspace{0.2ex}
\begin{equation}
    \begin{gathered}
    % \begin{aligned}
    y^f_{Y'} = x^f_{Y'} \quad \text{ } \quad y^f_U = x^f_U + t \quad \text{ } \qquad y^f_V = x^f_V + t
    \\[1.25ex]
    y_{Y'UV} = \text{IFFT}(y^f_{Y'UV})
    \\[1.25ex]
    y = \text{Y'UV2RGB}(y_{Y'UV})
    % \label{eq:wml-1}
    % \end{aligned}
    \end{gathered}
\end{equation}
\vspace{0.2ex}

where IFFT($x$) finds the inverse fast fourier transform of $x$ and Y'UV2RGB($x$) converts x from $Y'UV$ color space to $RGB$ color space. Since $t$ is in frequency space, the residual $r$ (defined as $y - x$) is symmetric and spatial transformation invariant. A model $F_\theta$ learns the presence of $r$ instead of $x$ as a unique identifier pattern for the target class (Sec. \ref{subsec:blur}). 

\begin{figure*}[tp]
    \centering
    \includegraphics[width=0.9\textwidth]{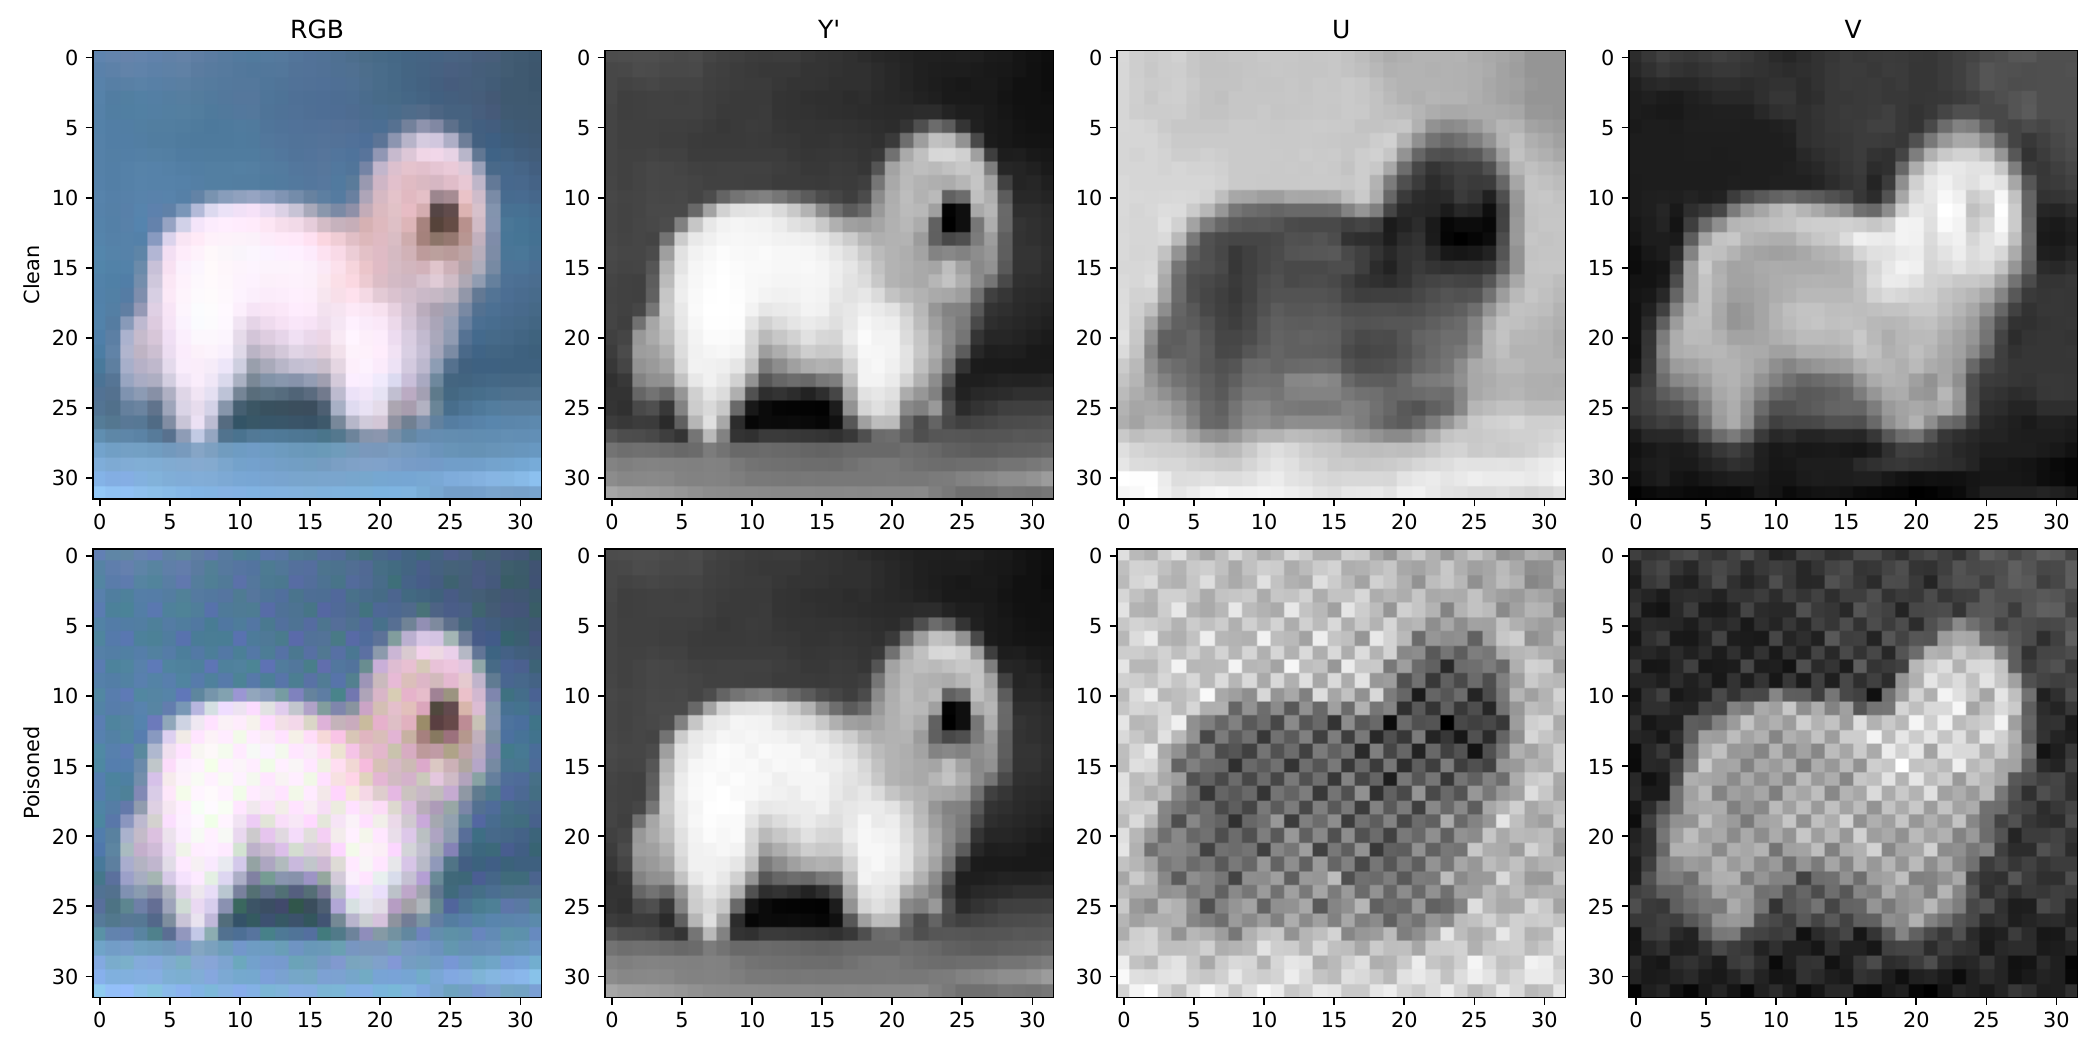}
    \caption{Effect of the CTRL poisoning on chroma and luma channels. As it is apparent, the luma channel (Y') remains unaffected from the poisoning while the chroma channels (U and V) are heavily distorted}
    \label{fig:ctrl-luma}
\end{figure*}
