# Supplementary material for: Towards Adversarial Robustness And Backdoor Mitigation in SSL
Source: arXiv:2403.15918 source file (2024-09-16)
Supplement: Supplementary file 3 [file blur.tex]

\subsection{Blur and frequency-based attacks}
\label{sec:app_blur}

Consider a clean image $x$ and its poisoned variant $y$. Let their blurred forms be represented as $x_b$ and $y_b$. Considering our threat model (Sec. \ref{sec:method}), an attacker can poison a fraction of the dataset. A potent backdoor attack would try to minimize the variance of trigger pattern while maintaining evasiveness. Generalizing dependence on $x$, let the trigger pattern in the frequency domain be represented as $t(x)$. For FIBA and CTRL, $t(x)$ is defined as:
% \begin{equation}
\begin{gather}
    \begin{aligned}
    \text{CTRL} : t_{i, j}(x): & \left
        \{\begin{array}{c l}
        c & \hspace{0.5em} i = j \text{ and } i \in \{\frac{s}{2}, s\}\\
        0 & \hspace{0.5em} \text{otherwise}
        \end{array} 
        \right.
        % & \hspace{0.5em}
    \\[2ex]
    \text{FIBA} : t_{i,j}(x): & \left
        \{\begin{array}{c l}
        \mathcal{M}ag(x^f) & \hspace{0.5em} (i, j) \in \text{ low freq. patch}\\
        0 & \hspace{0.5em} \text{otherwise}
        \end{array} 
        \right.
        % & \hspace{0.5em}
    \end{aligned}
\end{gather}

 where $\mathcal{M}ag$(x) finds the maginute of the complex number $x$. Poisoned image $y(x)$ is obtained as $\text{IFFT}(x^f + t(x))$.  Blurred image $x_b$ is obtained using a blur kernel $k$ as $k * x$. Now $y_b$:
\begin{gather}
    \begin{aligned}
    y_b &= k * y \\
                &= k * \text{IFFT}(x^f + t(x)) \\
                &= \text{IFFT}(k^f\cdot x^f + k^f\cdot t(x))\\
                &= \text{IFFT}(k^f \cdot x^f) + \text{IFFT}(k^f \cdot t(x))\\
                &= x_b + \describe{k * \text{IFFT}(t(x))}{trigger}
    % \label{eq:ifft}
    \end{aligned}
\end{gather}
where, $k^f$ represents FFT($k$). As discussed in Sec. \ref{subsec:FIBA}, FIBA already has a poor ASR in SSL due to the variance present in $t(x)$. In CTRL $t(x)$ is not entirely independent of $x$. The authors \emph{clamp} $y$ to lie between $\left[0, 1\right]$, which is a non-linear operation. Therefore, the residual $r(x) = y - x$ (Fig. \ref{fig:ctrl-residuals}) varies with the image $x$. When $r(x)$ is blurred to get $r_b(x)$, its dependence (indicated by variance) on $x$ is amplified. Even without clamp, randomly sampling blur strength adds enough variance in the residual $r_b(x)$ to impede its association with the target class instead of $x_b$.

\begin{figure*}[tp]
    \centering
    \begin{minipage}[b]{0.75\textwidth}
        \centering
        \includegraphics[width=\textwidth]{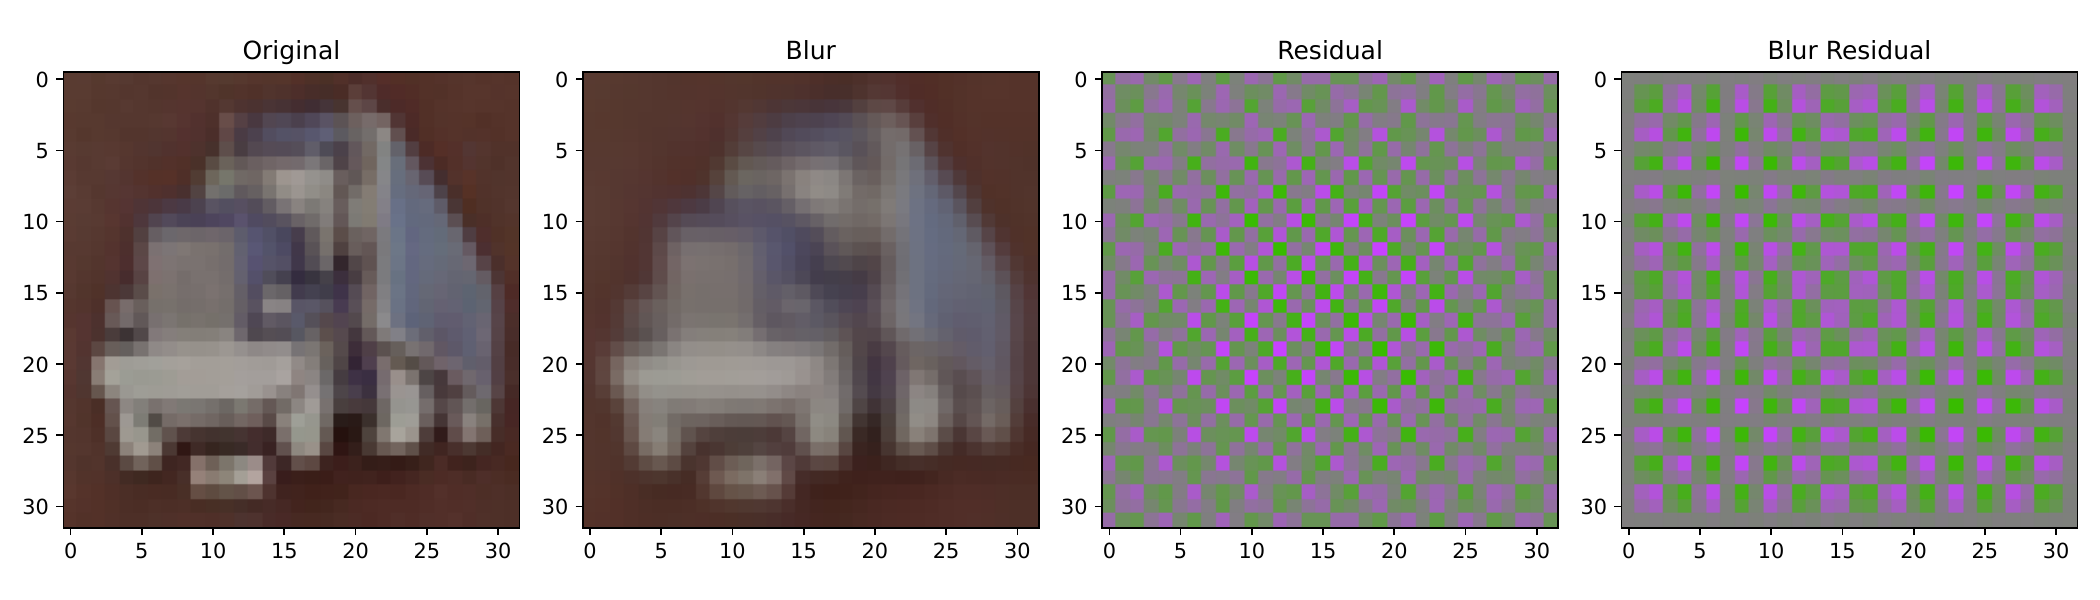}
    \end{minipage}
    \begin{minipage}[b]{0.75\textwidth}    
        \vspace{-3ex}
        \centering
        \includegraphics[width=\textwidth]{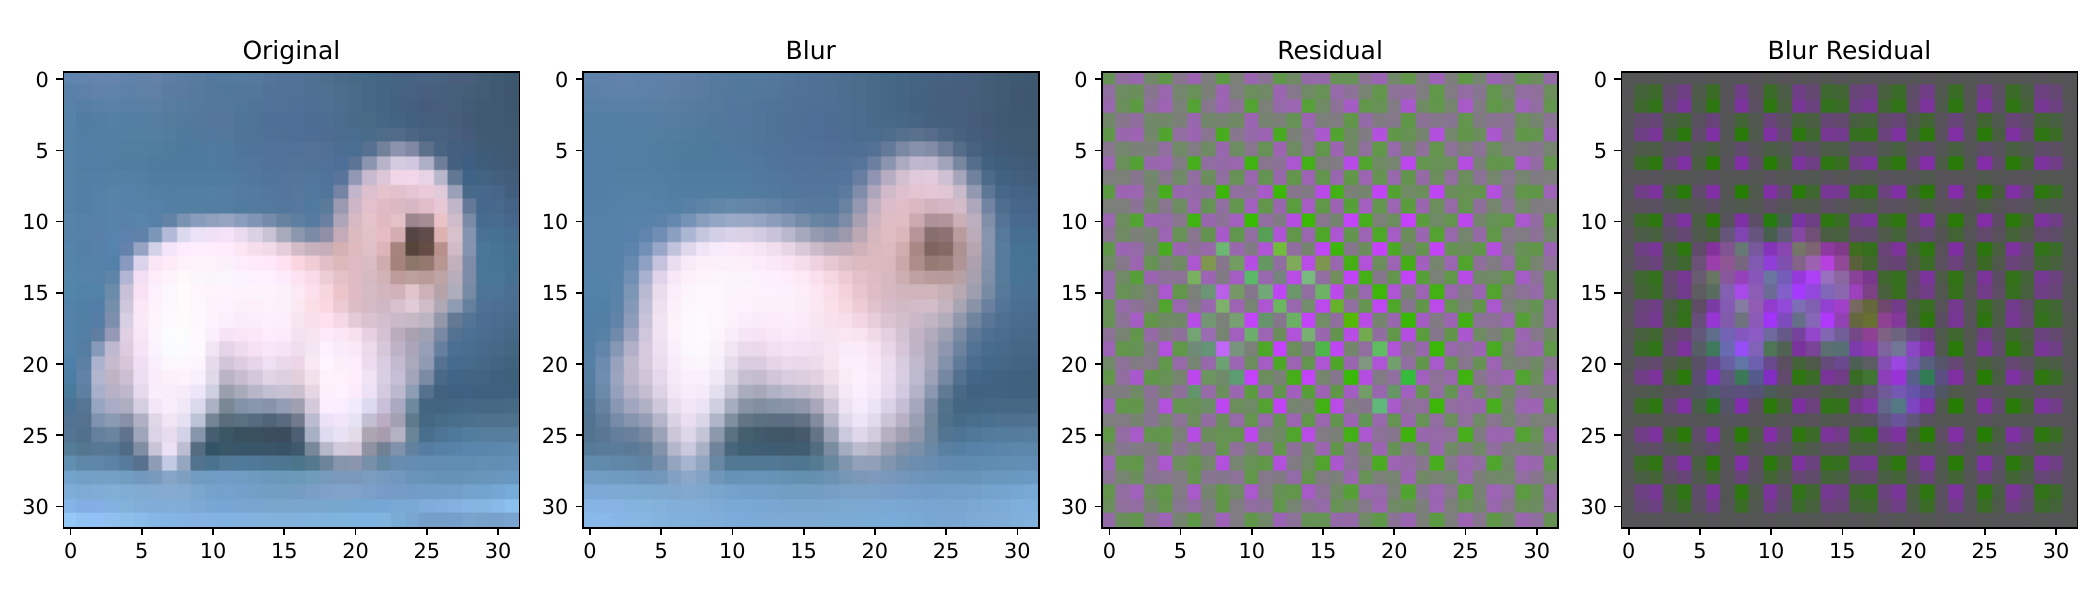}
    \end{minipage}
    \caption{Example of CTRL attack on two different images. The residual $r$ remains mostly identical for different images, thereby providing a path of least variance. Blurring the poisoned image $y$ results in a residual $r_b$ which varies between images.}
    \label{fig:ctrl-residuals}
    \vspace{-1ex}
\end{figure*}
